# Supplementary material for: Impact of Dynamical Tides on the Reconstruction of the Neutron Star Equation of State
Source: arXiv:2109.07566 source file (2022-09-27)
Supplement: Supplementary file 1 [file suppl.tex]

%%%%% SUPPLEMENTAL MATERIAL
\section{Supplemental Material}
Given a set of observations, we can construct the Bayesian odds ratio between competing models $M_i$. The posterior probability for a model $M_i$ can be written as
\begin{align} 
    P(M_i | d, I) &= \frac{P(M_i|I) P(d|M_i , I)}{P(d|I)},
\end{align}
where $P(H_i|I)$ is the prior probability on the model and $P(d|I)$ is the prior probability of the data. The odds ratio between two models $M_i$ and $M_j$ is defined by
\begin{align}
    \mathcal{O}_{ij} &= \frac{P(M_i|d,I)}{P(M_j|d,I)} = \frac{P(M_i|I)}{P(M_j|I)} \frac{P(d|M_i,I)}{P(d|M_j,I)} .
\end{align}
For a population of $N$ detections the odds ratio is simply 
\begin{align}
    \mathcal{O}_{ij} &= \frac{P(M_i|I)}{P(M_j|I)} \prod_{n=1}^{N}  \frac{P(d|M_i,I)}{P(d|M_j,I)} .  
\end{align}
Here we consider two models, one model incorporating dynamical tidal corrections and the other model using only adiabatic tidal terms. Although dynamical tides are a robust theoretical prediction, in the absence of additional information we assume that both models are a priori equally likely, $P(M_i|I) = P(M_j|I)$. For the population of binaries considered in this paper, we find overwhelming support in favour of the model containing dynamical tides in ET. For the population of binaries observed in the O5 detector network, we do not find significant support for the dynamical hypothesis with the odds ratio being relatively uninformative, despite the observed systematic biases.

% Odds ratios
\begin{figure}[h!]
\label{fig:odds}
\includegraphics[width=\columnwidth]{./Figures/odds.pdf}
\caption{Odds for $50$ BNS events in ET.}
\end{figure}

\begin{figure}[h!]
\label{fig:odds}
\includegraphics[width=\columnwidth]{./Figures/N_odds.pdf}
\caption{Odds for $50$ BNS events in ET.}
\end{figure}

\clearpage

%\end{document}

\begin{table}[]
\setlength{\tabcolsep}{3.pt}
    \centering
    {
    \begin{tabular}{c|c|c c c}
    \hline 
    \hline 
        $\mathcal{M}_c\, [M_\odot]$ & $M\, [M_\odot]$ & \multicolumn{3}{c}{$\tilde{\Lambda}$} \\
        & & APR4 & SLy & MPA1 \\
        \hline 
         0.948847 & 2.188 & 1080.91 & 1460.95 & 1997.16  \\
         1.067453 & 2.4615 & 553.06 & 745.07 & 1067.99 \\
         1.186058 & 2.735 & 293.50 & 392.48 & 595.21  \\
         1.304664 & 3.0085 & 159.25 & 210.37 & 341.90 \\
         1.423270 & 3.282 & 87.12 & 112.95 & 200.52 \\
         1.541876 & 3.5555 & 47.25 & 59.43 & 118.99 \\
         1.660481 & 3.829 & 24.72 & 29.08 & 70.76 \\
         \hline
         \hline 
    \end{tabular}
    }
    \caption{\patricia{We can always remove it but it helps me when writing.}}
    \label{tab:my_label}
\end{table}
